# Supplementary material for: Extreme Relative Pose Estimation for RGB-D Scans via Scene Completion
Source: arXiv:1901.00063 source file (2019-01-05)
Supplement: Supplementary file 1 [file 06_appendix.tex]

\section{Global Convergence of Truncated Rotation Fitting}
\label{Section:Rotation:Fitting}

Consider $n$ point-pairs $(\bs{p}_i, \bs{q}_i), 1\leq i \leq n$. With $w_i$ we denote the weight associated with $(\bs{p}_i, \bs{q}_i)$. Our goal is find a rotation that fits the point-pairs. We shall employ truncated least squares
